# Supplementary material for: Ridge Rider: Finding Diverse Solutions by Following Eigenvectors of the Hessian
Source: arXiv:2011.06505 source file (2020-11-12)
Supplement: Supplementary file 1 [file appendix-algorithm.tex]

\section{Algorithms}

\begin{algorithm}[H]
\SetAlgoLined
\caption{Approximate Ridge Riding}
% \KwResult{}
\textbf{Input:} Numbers $N$ of rides, $R$ ridges considered per ride, $T$ max iterations per ridge, $S$ inner steps. \\
\textbf{Initialize:} Neural network $f_{\bm{\theta}}$ with $\bm{\theta}$ initialized to constant $\epsilon$ to be symmetric. \\
\For{$1$  to  N} {
  // Find a ridge. \\
  Sample random integer $r \in [1, R]$ and mini-batch ($\bm{x}, \bm{y}$).\\
  Use the power method to find the $r$-th most negative eigenvalue $\lambda$ and its eigenvector $\bm{e}$. \\
  Compute gradient $\bm{g} = \frac{\partial }{\partial \bm{\theta}} L\left(\bm{y}, f_{\bm{\theta}}(\bm{x})\right)$ and set ridge $\bm{e} = \text{sign}(\bm{e} \cdot \bm{g}) \bm{e}$. \\
  
  // Follow the ridge. \\
  \For{$1$ to T} {
    % $e = e / \norm{e}_2$ \\
    $\bm{\theta}_{old} = \bm{\theta}$ \\
    $\bm{\theta} = \bm{\theta} - lr_{\bm{\theta}}~ \bm{e} $ \\
    $\lambda = \lambda +  \bm{e}^T (\mathcal{H}(\bm{\theta})- \mathcal{H}(\bm{\theta}_{old})) \bm{e} $ \\

    // Update eigenvalue and eigenvector. \\
    Sample a mini-batch $\bm{x}, \bm{y}$. \\
    \For{$1$ to S} {
      // Use gradient descent to find: \\
      $\lambda, \bm{e} = \argmin_{\lambda, \bm{e}} L(\bm{e}, \lambda ; \bm{\theta}) = \argmin_{\lambda, \bm{e}} (\norm{(1/\lambda) \mathcal{H}(\bm{\theta})\bm{e} / \norm{\bm{e}}_2 - \bm{e} / \norm{\bm{e}}_2}_2^2)$.
    }
  }
 }
 \label{algorithm:rr}
\end{algorithm}
